# Supplementary material for: The Hitchhiker's Guide to Malicious Third-Party Dependencies
Source: arXiv:2307.09087 source file (2023-10-06)
Supplement: Supplementary file 1 [file appendix.tex]

\section{Countermeasures}

\begin{table*}[!htp]
	% Green: \cellcolor[HTML]{98FB98}
	% Yellow: \cellcolor[HTML]{FBB917}
	% Red: \cellcolor[HTML]{FF0000}
	
	\centering
	\begin{adjustbox}{angle=0}
		\begin{tabular}{r|ccc|}
			\toprule
			
			%\rowcolor[HTML]{9B9B9B} 
			% \multicolumn{3}{c}{\textbf{How to achieve \acl{ACE}}} \\ \cmidrule(lr){1-3}  
			\multicolumn{1}{c}{\textbf{Recommendations to prevent \ac{ACE} from 3rd-party libraries}} & \multicolumn{1}{p{1.5cm}}{\textbf{Technique(s) Addressed}} \\ \cmidrule(lr){1-1} \cmidrule(lr){2-2}  
			
            \multicolumn{1}{p{15cm}}{(\textbf{Rec-0}) Check the presence of install hooks keywords (e.g., \texttt{pre-install} in \textit{package.json}) for all dependencies (direct and transitive).} & \multicolumn{1}{p{1cm}}{I1}  \\

			\multicolumn{1}{p{15cm}}{(\textbf{Rec-1}) Ignore execution of commands/scripts specified in install hooks for all dependencies (direct and transitive).} & \multicolumn{1}{p{1cm}}{I1}  \\

            \multicolumn{1}{p{15cm}}{(\textbf{Rec-2}) Review content of commands/scripts specified in install hooks for all dependencies (direct and transitive).} & \multicolumn{1}{p{1cm}}{I1}  \\

            \multicolumn{1}{p{15cm}}{(\textbf{Rec-3}) Prefer pre-built distributions over source distributions for all dependencies (direct and transitive).} & \multicolumn{1}{p{1cm}}{I1; I2}  \\

            \multicolumn{1}{p{15cm}}{(\textbf{Rec-4}) Check the presence of install script (e.g., \textit{setup.py}) for all dependencies (direct and transitive).} & \multicolumn{1}{p{1cm}}{I2}  \\

            \multicolumn{1}{p{15cm}}{(\textbf{Rec-5}) Review the content of install script (e.g., \textit{setup.py}) for all dependencies (direct and transitive).} & \multicolumn{1}{p{1cm}}{I2}  \\

            \multicolumn{1}{p{15cm}}{(\textbf{Rec-6}) Check the presence of build extensions for all dependencies (direct and transitive).} & \multicolumn{1}{p{1cm}}{I3; B1}  \\

            \multicolumn{1}{p{15cm}}{(\textbf{Rec-7}) Review the content of scripts related to build extensions for all dependencies (direct and transitive).} & \multicolumn{1}{p{1cm}}{I3; B1}  \\

            \multicolumn{1}{p{15cm}}{(\textbf{Rec-8}) Check the presence of build scripts for all dependencies (direct and transitive).} & \multicolumn{1}{p{1cm}}{I3; B2}  \\

            \multicolumn{1}{p{15cm}}{(\textbf{Rec-9}) Review the content of build scripts for all dependencies (direct and transitive).} & \multicolumn{1}{p{1cm}}{I3; B2}  \\

            \multicolumn{1}{p{15cm}}{(\textbf{Rec-10}) Review the content of methods (e.g., \texttt{Init\_<extension-name>()} in Ruby) or scripts (e.g., \texttt{\_\_init\_\_.py} in Python) which are executed at import time.} & \multicolumn{1}{p{1cm}}{R1}  \\

            \multicolumn{1}{p{15cm}}{(\textbf{Rec-10}) Review the content of constructor or methods imported from 3rd-party libraries.} & \multicolumn{1}{p{1cm}}{R2; R3}  \\

            \multicolumn{1}{p{15cm}}{(\textbf{Rec-11}) Check and analyze the usage of monkey-patching in imported 3rd-party libraries.} & \multicolumn{1}{p{1cm}}{R4}  \\

            \multicolumn{1}{p{15cm}}{(\textbf{Rec-12}) Check and analyze any replacement of invoked functions at runtime through function/API hooking techiques.} & \multicolumn{1}{p{1cm}}{R4}  \\

            \multicolumn{1}{p{15cm}}{(\textbf{Rec-13}) Check and analyze the code of the tests to be run.} & \multicolumn{1}{p{1cm}}{T1}  \\

            \multicolumn{1}{p{15cm}}{(\textbf{Rec-14}) Isolate environment when installing or building 3rd-party dependencies.} & \multicolumn{1}{p{1cm}}{I1; I2; I3; B1; B2}  \\

            \multicolumn{1}{p{15cm}}{(\textbf{Rec-15}) Analyze suspicious system calls and/or spawning of processes when installing or building 3rd-party dependencies.} & \multicolumn{1}{p{1cm}}{I1; I2; I3; B1; B2}  \\

            \multicolumn{2}{c}{}\\ \cmidrule(lr){1-2}

            \multicolumn{1}{c}{\textbf{Recommendations concerning evasion strategies}} & \multicolumn{1}{p{1.5cm}}{\textbf{Technique(s) Addressed}} \\ \cmidrule(lr){1-1} \cmidrule(lr){2-2}  

            \multicolumn{1}{p{15cm}}{(\textbf{Rec-14}) Highlight the presence of non-human-readable strings that could indicate usage of encoding, encryption, or compression.} & \multicolumn{1}{p{1cm}}{SO-1; SO-3; SO-4}  \\

            \multicolumn{1}{p{15cm}}{(\textbf{Rec-15}) Check the presence of binary arrays and reverse-engineer their content to check if they do not contain suspicious strings.} & \multicolumn{1}{p{1cm}}{SO-3;}  \\

            \multicolumn{1}{p{15cm}}{(\textbf{Rec-16}) Highlight the presence of concatenation of strings (e.g., leveraging data-flow analysis).} & \multicolumn{1}{p{1cm}}{SO-5}  \\

            \multicolumn{1}{p{15cm}}{(\textbf{Rec-17}) Raise suspicion when encountering non-readable names in identifiers.} & \multicolumn{1}{p{1cm}}{CO-1}  \\

            \multicolumn{1}{p{15cm}}{(\textbf{Rec-18}) Raise suspicion when encountering encoded, compressed, or encrypted code.} & \multicolumn{1}{p{1cm}}{CO-2; CO-3; CO-4}  \\

            \multicolumn{1}{p{15cm}}{(\textbf{Rec-19}) Highlight the presence of sensitive file extensions in 3rd-party packages (e.g., executables, shell scripts).} & \multicolumn{1}{p{1cm}}{}  \\

            \multicolumn{1}{p{15cm}}{(\textbf{Rec-20}) Highlight the presence of large numbers of whitespaces (e.g., new lines, tabs).} & \multicolumn{1}{p{1cm}}{CO-10}  \\
			
			\bottomrule
		\end{tabular}
	\end{adjustbox}
	\caption{ aa }
	\label{tab:recommendations}
\end{table*}
